# Supplementary material for: Softmax Bias Correction for Quantized Generative Models
Source: arXiv:2309.01729 source file (2023-09-04)
Supplement: Supplementary file 1 [file 99_appendix.tex]

% \section*{Supplementary materials}
% \subsubsection*{A. Per attention head based bias correction}

% \begin{figure}[H]
%     \centering
%     \includegraphics[width=0.42\textwidth]{images/sm_output_graphic.png}

%     \caption{softmax output tensor, $\mathbf{Y} \in {\rm I\!R}^{heads \times L_{y} \times L_{x} }$, with softmax applied along the highlighted dimension}
%     \label{fig:SMoutput}
% \end{figure}

% In section 3.2, we discussed how we can calculate the per tensor correction factor using the calibration set $\mathcal{X}$ for each softmax layers in the networks. Expanding on similar lines, we define per attention head correction factor as


% \begin{gather}
%       \nonumber\lambda_{i} = \frac{1 - \mathbf{E}_{x} \left[ \sum_{j}^{L_{y}} \sum_{k}^{L_{x}} softmax \left( \mathbf{X_{i,j,k}} \right) \right]}{L_{x}}
% \end{gather}

% where, $\lambda_{i}$ as the $i^{th}$ attention head correction factor.

% \subsubsection*{B. Additional experimental results}

% \begin{table}[h!]
%     % \addtolength{\tabcolsep}{-2pt}
%     \centering
%     % \fontsize{8.25pt}{9.25pt}\selectfont
%     \fontsize{9.25pt}{9.25pt}\selectfont
%     \begin{tabular} {  lcccc }
%     \toprule
%     Activation in 8 bits & SQNR($\uparrow$) \\
%     \midrule
%     None~(baseline) & $9.66$\\
%     Query(Q) & $9.59$ \\
%     Key(K) & $9.66$ \\
%     Value(V) & $9.66$\\
%     Attention scores (input to softmax)
% & $9.60$ \\
%      Softmax & $2.85$ \\
%     \bottomrule
% \end{tabular}
% \caption{Quantization sensitivity analysis for attention layers in the denoising U-Net of stable diffusion. We quantize one tensor to 8 bit while keeping the rest in W8A16 and report mean SQNR.($\uparrow$): the higher, the better.} 
%     \label{tab:attn_sensitivity_analysis_W8A16}
% \end{table}

% We expand our experiments to include weight quantization to showcase biased nature of the quantized softmax output also prevalent in W8A16 model. Similar to table \ref{tab:attn_sensitivity_analysis} and \ref{tab:performance}, we report the sensitivity analysis and improvements gained using per tensor and per attention head based correction in \ref{tab:attn_sensitivity_analysis_W8A16} and \ref{tab:performance_W8A16}. 

% \begin{table}[t]
%     \addtolength{\tabcolsep}{-4pt}
%     \centering
%     \fontsize{9.25pt}{9.25pt}\selectfont
%     % \fontsize{8.00pt}{8.25pt}\selectfont

%     \begin{tabular} {  lccc }
%     \toprule    Correction axis & SD (SQNR$\uparrow$) & OPT (ppl$\downarrow$) \\
%     \midrule
%     None & $2.85$ & $-$ \\
%     Tensor & $5.30$ & $-$ \\
%     Attention Head & $5.23$ & $-$ \\
%     \bottomrule
% \end{tabular}
%     \caption{Effect of bias correction along different softmax ouput axes. We report SQNR for Stable Diffusion (SD) and CLM perplexity for OPT. ($\uparrow$): the higher, the better; ($\downarrow$): the lower, the better.} 
%     \label{tab:performance_W8A16}
% \end{table}
